# Supplementary material for: Adaptive Simulation-based Training of AI Decision-makers using Bayesian Optimization
Source: arXiv:1703.09310 source file (2017-07-28)
Supplement: Supplementary file 1 [file Appendices.tex]

\section*{Appendix A -- Kernels}
discuss different kernels and properties

\section*{Appendix B -- Acquisition Functions}
Add stuff here?

\section*{Appendix C -- Hyperparameter Learning}\label{sec:HP_learning}

MAP was the most stable and tolerant of different objective functions and simulation settings. Both MLE and cross-validation were very sensitive and tended to over-fit the training data\footnote{A fact caused by the fact that we are trying to minimize the number of function evaluations}. This is undesirable, for if the hyperparameters are selected poorly (yielding a GP surrogate function that does not reflect the true objective funciton ``well enough'') the BO will begin searching in the wrong places. Despite the use of MAP, there are still some conditions presenting stability difficulties. Future efforts will investigate Monte-Carlo methods and use distributions over the hyperparameters instead of explicitly choosing the best estimate.

\paragraph{Maximum likelihood estimate (MLE): }\label{MLE}

A maximum likelihood estimate (MLE) maximizes the probability of the model given the data, model and hyperparameters. Specifically, it involves finding the maximum value, $\Theta$, of the distribution $p(y|X,\Theta,H_{i})$(see equation 7 which applies for a Gaussian likelihood) and selects that value for the hyperparameters. Gradient descent can then be used to descend the gradient of the likelihood.

One drawback with this approach is that it is prone to overfitting~\cite{Cawley2010,Rasmussen2006}. This can be a significant problem especially when trying to minimize the number of experiments or when there are many hyperparameters.

\paragraph{Cross-Validation: }\label{CV}

Another way to select the hyperparameters is to use cross-validation. Cross validation refers to the process where some portion of the experimental data is held out for testing. The goal is to choose parameters that generalize well to ``test'' data. Although cross-validation has zero bias (in expectation it will estimate the true parameters), it has a large variance. This makes it unreliable when selecting hyperparameters.

\paragraph{MAP: }
When using non-Gaussian hyperpriors the MMLE cannot be computed analytically. Instead variational inference approximations can be used to approximate the marginal likelihood with a simpler analytical result that is statistically ``close'' to the true results (in the sense of the Kullback-Leibler divergence between the approximate and true posterior probability distributions).

\section*{Appendix D -- Parallel Sampling}
\paragraph{two strategies for MAPS}
With respect to the implementation of MAPS, we experimented with two different strategies. The first is to sample multiple times at each maximum point of the acquisition function. For example, if the acquisition function recommends sampling at $x=2$, then we sample that location multiple times and treat all outcomes separately in the GP as independent data points. The second method is to sample the location ($x=2$ in our example) multiple times but only use the mean outcome in the GP over all the multiple samples.

Figure \ref{fig:mean_sampling} is the result of using mean sampling. It is using the same scenario as Figure \ref{fig:multiple_sampling} but using only the mean of the multiple samples in the kernel. The key point is that fitting the mean of the objective function at a point is different than fitting the individual outcomes of the objective function at that point. It seems in our application that mean sampling smooths the variation too much and was not able to fit the true objective very well.

\begin{figure}[htbp]
    \centering
    \includegraphics[width=0.85\textwidth]{Figures/MeanSample.png}
    \caption{Example of averaging multiple evaluations of the objective function and putting that into the kernel}
    \label{fig:mean_sampling}
\end{figure}

Figure \ref{fig:multiple_sampling} is an example of taking multiple samples on each evaluation. This method has worked very well in our experiments. It is able to take enough samples to give the GP some idea of the inherent uncertainty in the system.

\begin{figure}[htbp]
    \centering
    \includegraphics[width=0.85\textwidth]{Figures/MultipleSample.png}
    \caption{Example of taking multiple samples at each location and incorporating those directly into the GP.}
    \label{fig:multiple_sampling}
\end{figure}

\paragraph{Regret based methods: }\label{regret-based-methods}

We have not investigated regret based methods, but they might prove useful in the TALAF problem. The idea of regret based sampling is to select multiple points but trying to maximize the possible reward in the future as opposed to choosing what will be best now (Snoek, Larochelle, and Adams).

\paragraph{Selecting multiple points to sample :}
There are several methods that can be used to sample multiple points in parallel. Thompson sampling is one such method that relies on the fact that a GP is a distribution over functions. A function can be drawn from a GP following the procedure in (Rasmussen and Williams 16). This method does not explicitly make use of an acquisition function. Instead multiple random functions are drawn from the GP and then the minimum of each function is selected as a candidate for the next experiments. Figure \ref{fig:thompson_sampling} is an illustration of what sampling functions from a one dimensional problem look like. While Thompson sampling works well in a 1-d case as the dimensionality increases it suffers because it is impractical to sample GPs in high-dimensional spaces with adequate resolution. This is because an entire function needs to be sampled simultaneously due to the points $f_{*}$ being jointly-Gaussian (see equations 8 and 9).

\begin{figure}[htbp]
    \centering
    \includegraphics[width=0.85\textwidth]{Figures/ThompsonSampling.png}
    \caption{Example of drawing 50 functions from a GP. The minimum of each function is calculated and then those locations are explored simultaneously in the next iteration of optimization.}
    \label{fig:thompson_sampling}
\end{figure}

\paragraph{Acquisition cluster sampling}\label{acquisition-cluster-sampling}

A second method we developed called ``Acquisition cluster sampling'' is based on adapting the expected improvement (EI) metric. Specifically, when using the DIRECT algorithm to optimize the EI acquisition function we store the evaluation points and then use DBSCAN ``density-based spatial clustering of applications with noise'' (DBSCAN) to find areas of interest (Ester et al.). Once we have identified these areas we then select several experiments in the neighborhood of each. This method has the advantage that it uses the output of DIRECT (which would be used in the standard EI evaluation). An example of the clustering is shown in Figure 8.

\begin{figure}[htbp]
    \centering
    \includegraphics[width=0.85\textwidth]{Figures/ClusterSampling.png}
    \caption{(a) Example of DBSCAN output on data obtained from DIRECT optimization. (b) The true objective function.}
    \label{fig:cluster_sampling}
\end{figure}

\subsubsection{Using a warped GP as the surrogate
function}\label{using-a-warped-gp-as-the-surrogate-function}

When confronted with an objective function with constraints it is possible to use something called a warped GP~\cite{Snelson2004}. The purpose is to warp the output of the objective function in a way that the GP will fit the constraints.

We have not implemented this approach in our current work on the TALAF problem. However, it would be critical when dealing with some objective functions (i.e. the time to kill should not be less than zero). We would like to re-visit the idea in the future so that we could allow objective functions that have constraints.
